# Supplementary material for: Learned Distributed Image Compression with Multi-Scale Patch Matching in Feature Domain
Source: arXiv:2209.02514 source file (2022-11-28)
Supplement: Supplementary file 1 [file appendix.tex]

\begin{figure*}[b]
	\centering
	\begin{minipage}[t]{0.05\linewidth}
		\rotatebox{90}{\Large  SI with brightness 1} \vspace{15pt}\\
		
		\rotatebox{90}{\Large  SI with brightness 1.5}
	\end{minipage}
	\begin{minipage}[t]{0.25\linewidth}
		\centering
		\includegraphics[width=\linewidth]{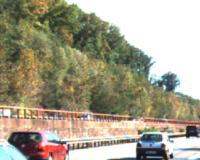}
		\centerline{SI}
		\centerline{}
		\vspace{-4pt}
		\\ 
		
		\includegraphics[width=\linewidth]{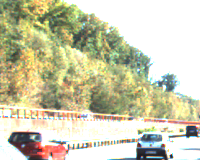} 
		\centerline{SI}
		\centerline{}
		
	\end{minipage}
	\!
	\begin{minipage}[t]{0.25\linewidth}
		\centering
		\includegraphics[width=\linewidth]{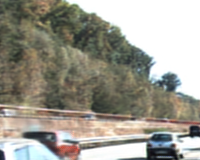} 
		\centerline{MSFDPM}
		\centerline{\fontsize{9pt}{\baselineskip}\selectfont0.0381/0.9392}
		\vspace{-4pt}
		\\ 
		\includegraphics[width=\linewidth]{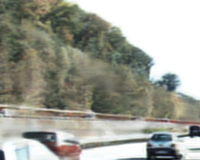} 
		\centerline{MSFDPM}
		\centerline{\fontsize{9pt}{\baselineskip}\selectfont0.0381/0.9188/38.13\%}
		
	\end{minipage}%
	\,
	\begin{minipage}[t]{0.25\linewidth}
		\centering
		\includegraphics[width=\linewidth]{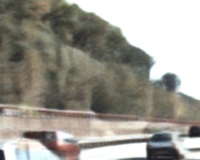} 
		\centerline{MSFDPM$_\text{img}$}
		\centerline{\fontsize{9pt}{\baselineskip}\selectfont0.0358/0.9047}
		\vspace{-4pt}
		\\ 
		\includegraphics[width=\linewidth]{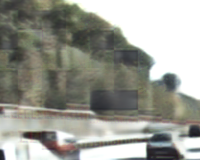} 
		\centerline{MSFDPM$_\text{img}$}
		\centerline{\fontsize{9pt}{\baselineskip}\selectfont0.0358/0.8863/96.84\%}
	\end{minipage}
	\centering
	\vspace{0pt}
	\caption{Visual comparisons of MSFDPM and MSFDPM$_\text{img}$ with brightness 1 and 1.5. Evaluation Metric is denoted by bpp/MS-SSIM/PR. } 
	\label{fig:feature_vs_image_visualization_brightness_10_and_15}
\end{figure*}

\section{Appendix A: Illustration of corresponding relationship of patches in different feature layers} 
\label{sec:appendix_A}

Fig. \ref{fig:toy_example_of_corresponding_patches} exhibits the detailed operations of the corresponding patches in different feature layers. 

\section{Appendix B: Supplementary Visualization of Robust Experiments} 
\label{sec:appendix_B}

Fig. \ref{fig:feature_vs_image_visualization_brightness_10_and_15} shows the visualization results when the brightness of the side information image changes. It can be seen that when the brightness is $1.5$, the example of MSFDPM$_\text{img}$ shows a  block effect while the example of MSFDPM does not. This may be because the change of brightness causes the corresponding patches cannot be accurately matched in the image domain. Fig. \ref{fig:feature_vs_image_visualization_brightness_10_and_06} shows more visualization results. 

\begin{figure}[htbp]
	\centering
	\includegraphics[width=0.8\columnwidth]{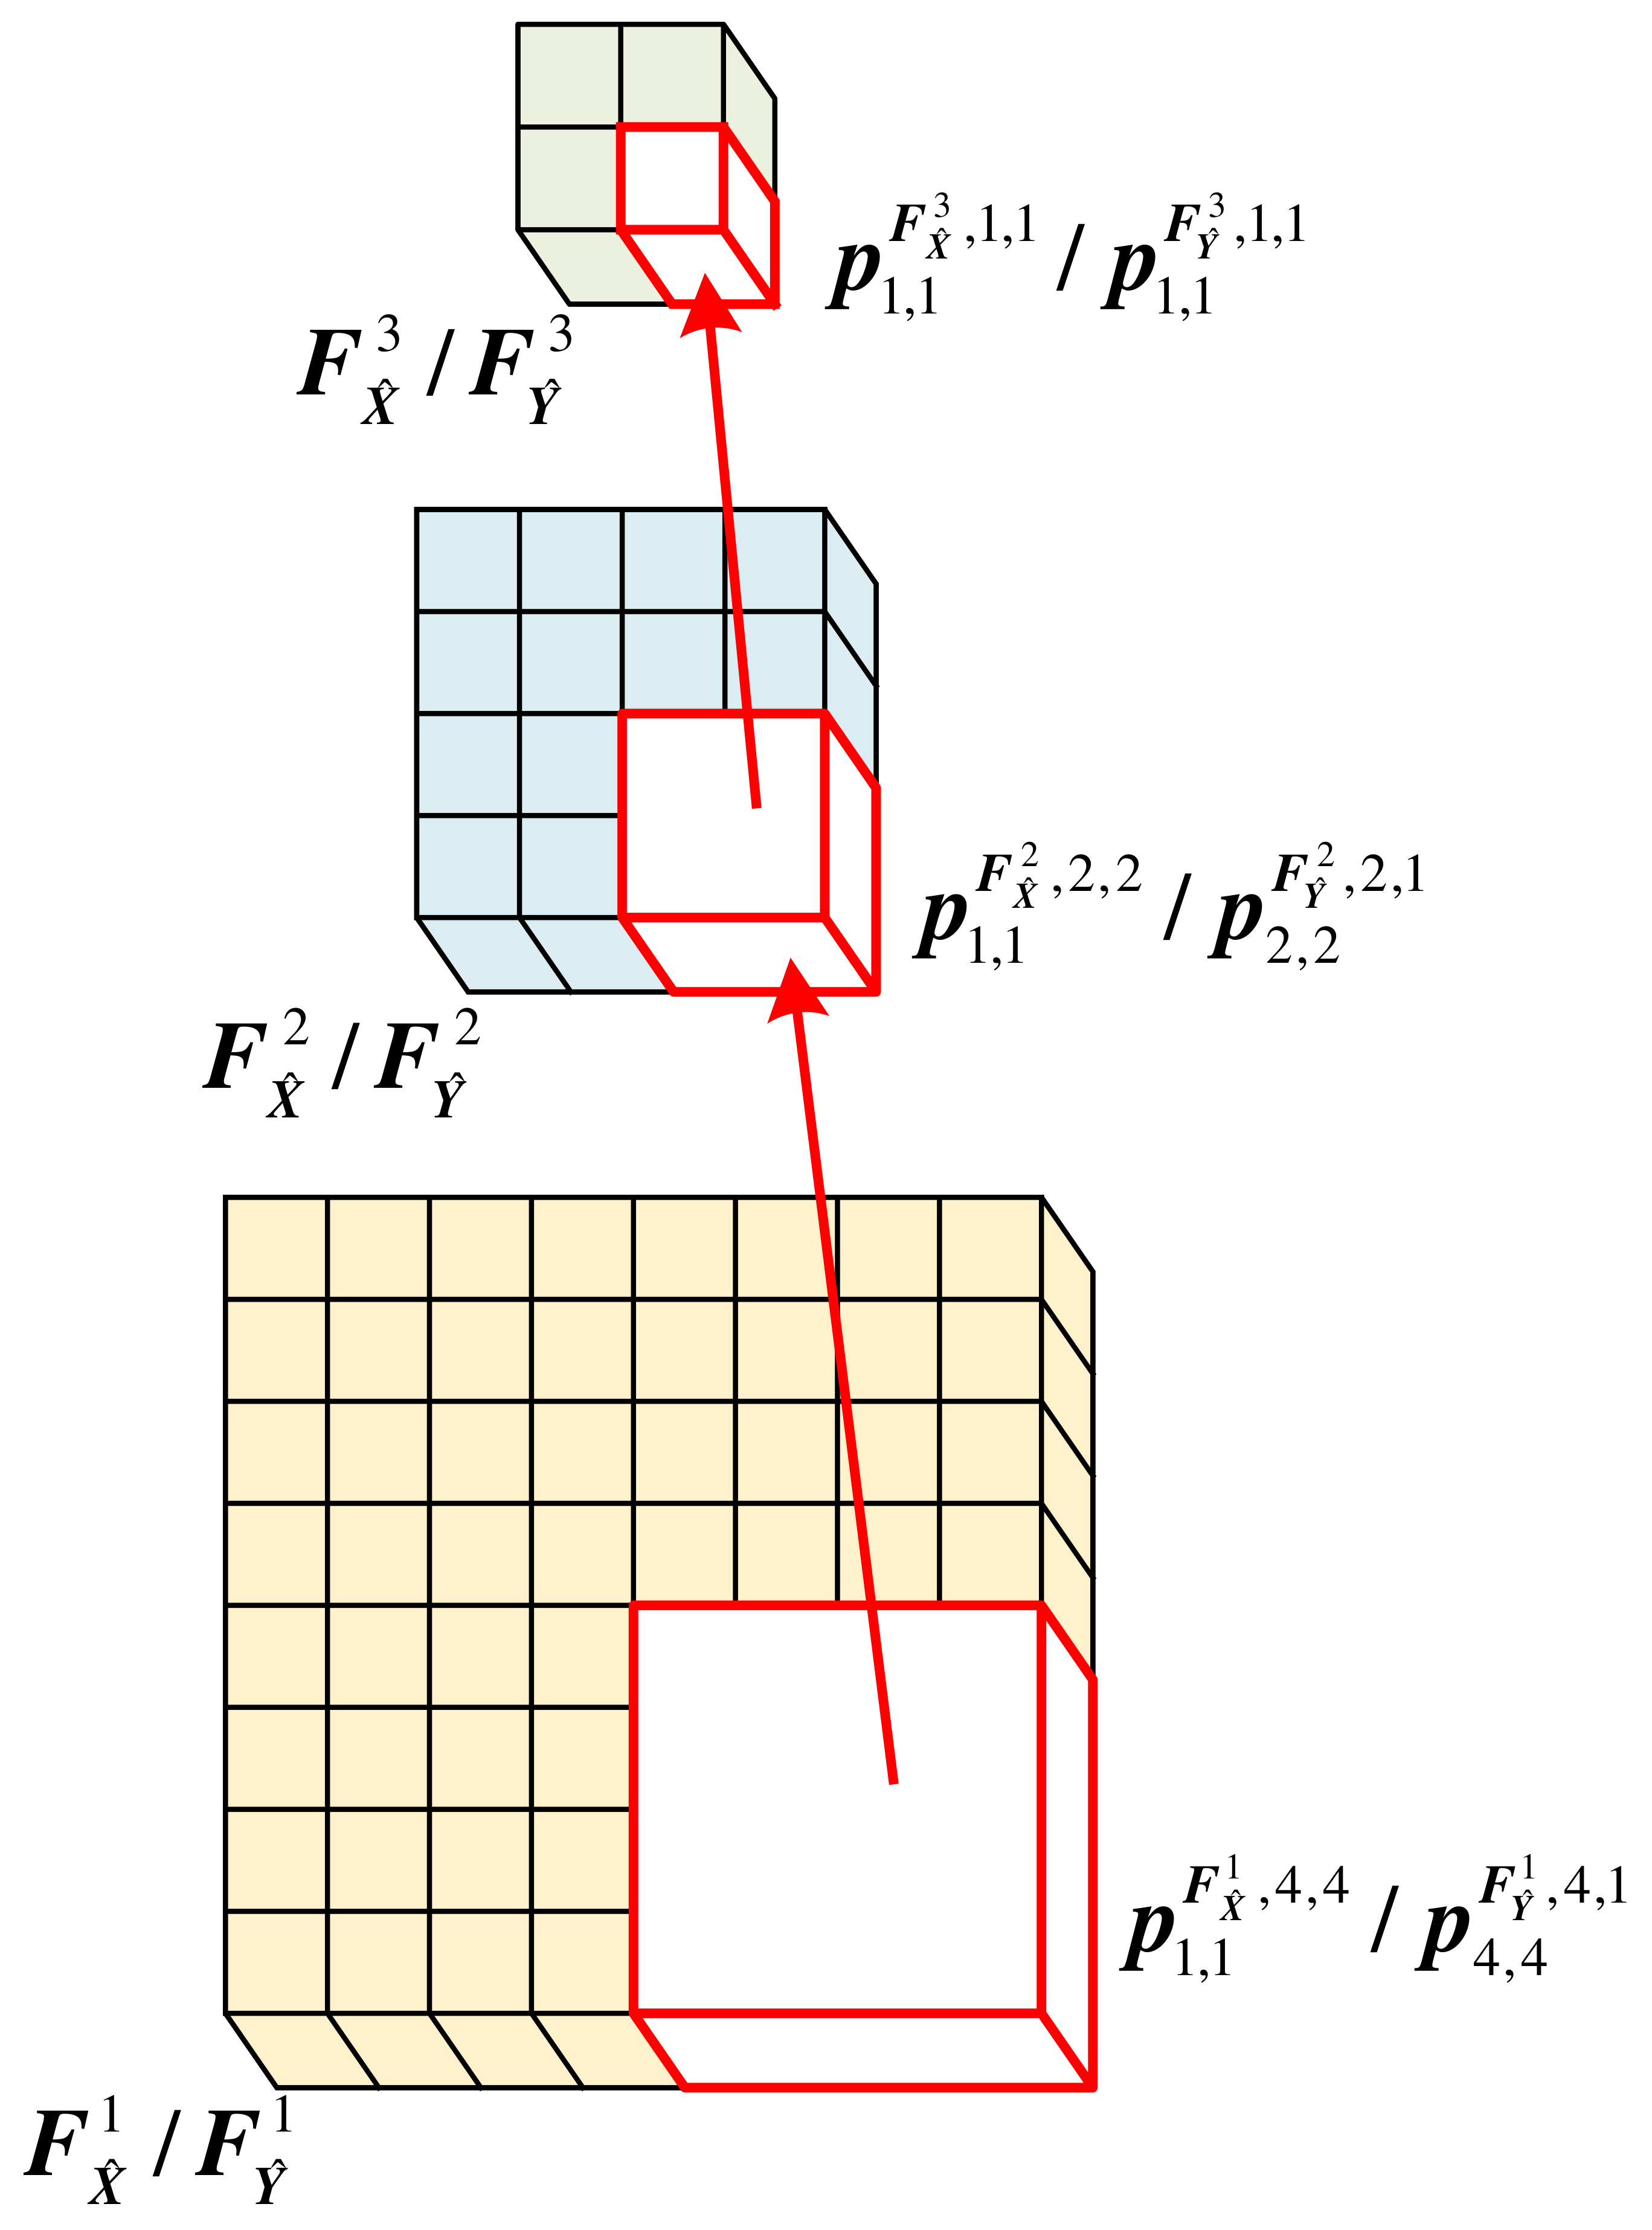}
	\caption{A toy example of the corresponding patches in different feature layers. 
	}
	\label{fig:toy_example_of_corresponding_patches}
\end{figure}

\begin{figure*}[t]
	\centering
	\begin{minipage}[t]{0.05\linewidth}
		\rotatebox{90}{\Large  SI with brightness 1} \vspace{15pt}\\
		
		\rotatebox{90}{\Large  SI with brightness 0.6} \vspace{15pt}
	\end{minipage}
	\begin{minipage}[t]{0.25\linewidth}
		\centering
		\includegraphics[width=\linewidth]{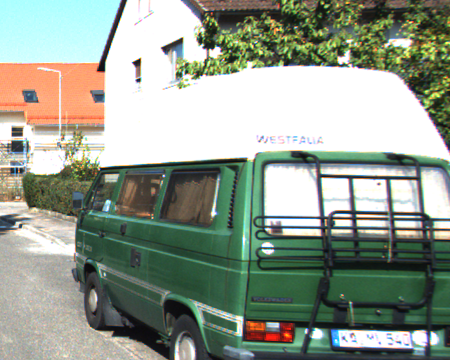}
		\centerline{SI}
		\centerline{}
		\vspace{-4pt}
		\\ 
		
		\includegraphics[width=\linewidth]{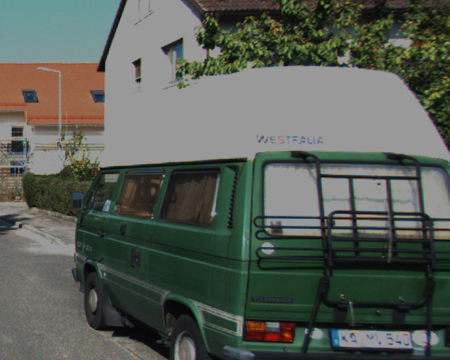} 
		\centerline{SI}
		\centerline{}
		
	\end{minipage}
	\!
	\begin{minipage}[t]{0.25\linewidth}
		\centering
		\includegraphics[width=\linewidth]{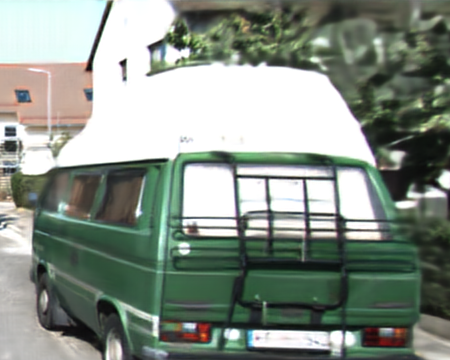} 
		\centerline{MSFDPM}
		\centerline{\fontsize{9pt}{\baselineskip}\selectfont0.0414/0.9172}
		\vspace{-4pt}
		\\ 
		\includegraphics[width=\linewidth]{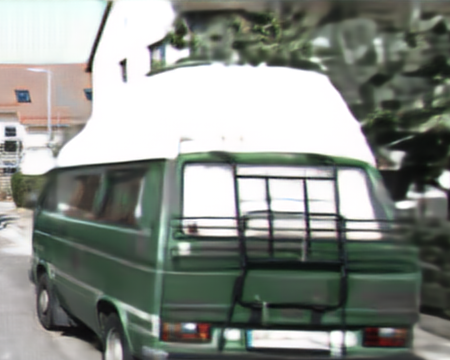} 
		\centerline{MSFDPM}
		\centerline{\fontsize{9pt}{\baselineskip}\selectfont0.0414/0.9059/34.98\%}

	\end{minipage}%
	\,
	\begin{minipage}[t]{0.25\linewidth}
		\centering
		\includegraphics[width=\linewidth]{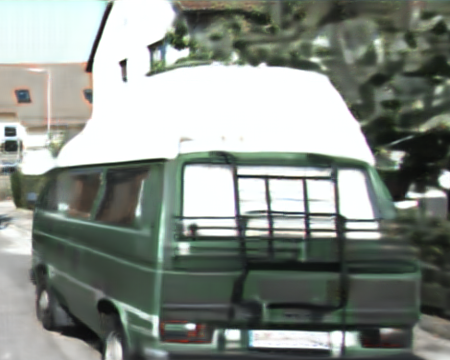} 
		\centerline{MSFDPM$_\text{img}$}
		\centerline{\fontsize{9pt}{\baselineskip}\selectfont0.0399/0.8936}
		\vspace{-4pt}
		\\ 
		\includegraphics[width=\linewidth]{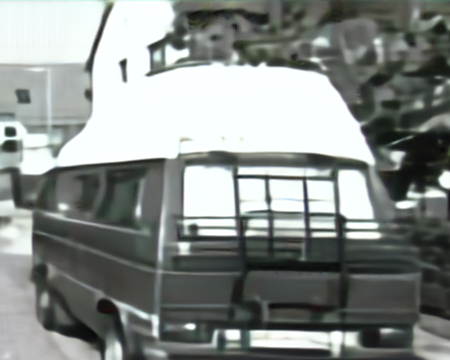} 
		\centerline{MSFDPM$_\text{img}$}
		\centerline{\fontsize{9pt}{\baselineskip}\selectfont0.0399/0.8846/103.45\%}
	\end{minipage}
	\centering
	\vspace{0pt}
	\caption{Visual comparisons of MSFDPM and MSFDPM$_\text{img}$ with brightness 1 and 0.6. Evaluation Metric is denoted by bpp/MS-SSIM/PR. } 
	\label{fig:feature_vs_image_visualization_brightness_10_and_06}
\end{figure*}

\section{Appendix C: Supplementary Ablation Experiments} 
\label{sec:appendix_C}

\begin{table}[th]
	\caption{The BD-Rate results of different MSFDPM variants. Baseline is single-image compression model (Cheng).}
	% The results in the subscript is the decrement of MAP compared to standard PHPQ. 
	\centering
	\resizebox{\columnwidth}{!}{
		\setlength{\tabcolsep}{.5em}{
			\begin{tabular}{lllll}
				\toprule
				\multirow{2}{*}{Variant} & \multicolumn{2}{c}{\emph{KITTI Stereo} }                             & \multicolumn{2}{c}{\emph{KITTI General}}                          \\
				\cmidrule(l){2-3} \cmidrule(l){4-5} 
				& BD-Rate$_\text{P}$ & BD-Rate$_\text{M}$ & BD-Rate$_\text{P}$ & BD-Rate$_\text{M}$\\
				\midrule
				
				MSFDPM & \textbf{-49.26\%}  & \textbf{-51.11\%}  & \textbf{-40.37\%}  & \textbf{-40.89\%}  \\
				
				MSFDPM$_{\text{vgg}}$  & -37.08\% & -29.35\%  & -18.80\% & -14.29\% \\
				
				MSFDPM$_{\text{w/o si}}$ & -0.33\% & -0.87\% & -1.33\% & -0.76\% \\
				
				\bottomrule
	\end{tabular}}}
	\label{tab:variants}
\end{table}

We design 2 more variants of MSFDPM:
(\textbf{i}) MSFDPM$_\text{vgg}$ replaces trainable feature extractor network with fixed VGG19 backbone to extract multi-scale side information features. 
(\textbf{ii}) MSFDPM$_\text{w/o si}$ doesn't input the aligned side information features into the feature fusion network. Experiment results are shown in Table \ref{tab:variants}. 
\begin{itemize}
	\item \textbf{Trainable Feature Extractor Network v.s. Fixed VGG19 Backbone.} MSFDPM outperforms MSFDPM$_\text{vgg}$ by an average BD-Rate$_\text{P}$ of $-16.88\%$ and an average BD-Rate$_\text{M}$ of $-24.18\%$. This demonstrates that the feature extractor trained for distributed compression is more suitable for extracting multi-scale side information features than the VGG19 pretrained for image classification task.
	\item \textbf{Feature Fusion Network with and without Side Information as Input.}
	MSFDPM outperforms MSFDPM$_\text{w/o si}$ by an average BD-Rate$_\text{P}$ of $-43.99\%$ and an average BD-Rate$_\text{M}$ of $-45.18\%$. In addition, MSFDPM$_\text{w/o si}$ barely has compression rate improvement compared with the single-image compression model. This indicates that side information rather than network structure dominates the compression rate improvement.
\end{itemize}
